# Supplementary material for: Highly Irregular Functional Generalized Linear Regression with Electronic Health Records
Source: arXiv:1805.08518 source file (2019-10-04)
Supplement: Supplementary file 1 [file appendix.tex]

\documentclass[../Draft_v02.tex]{subfile}
\begin{document}
%\input{appendix-concordance}

%---------------------------------------------------------------------------------%
%                                    Appendix                                     %
%---------------------------------------------------------------------------------%
\section{Additional Simulation Results}\label{sec:apptables}

% latex table generated in R 3.5.2 by xtable 1.8-4 package
% Tue Aug 13 13:49:18 2019
\begin{table}[!h]
\centering
\scalebox{1}{
\begin{tabular}{lllllllllllll}
  \hline
   N & \multicolumn{4}{c}{w = 0} & \multicolumn{4}{c}{w = 5} & \multicolumn{4}{c}{w = 10} \\ \cmidrule(lr){2-5}\cmidrule(lr){6-9}\cmidrule(lr){10-13}
  & MeC & MuC & MeU & MuU & MeC & MuC & MeU & MuU & MeC & MuC & MeU & MuU \\
 \hline
100 & 1.44 & 0.05 & 1.44 & 0.05 & 5.53 & 3.34 & 6.57 & 7.76 & 14.08 & 13.19 & 22.90 & 30.88 \\ 
  200 & 0.74 & 0.02 & 0.74 & 0.02 & 5.26 & 3.31 & 5.02 & 7.73 & 13.96 & 13.17 & 17.99 & 30.95 \\ 
  400 & 0.32 & 0.01 & 0.32 & 0.01 & 5.12 & 3.30 & 4.13 & 7.73 & 13.90 & 13.16 & 15.42 & 30.90 \\ 
  800 & 0.18 & 0.01 & 0.18 & 0.01 & 5.03 & 3.29 & 3.69 & 7.70 & 13.87 & 13.15 & 14.27 & 30.76 \\ 
   \hline
\end{tabular}
}
\caption{MISE as N increases, using true parameters, with J = 3.} 
\end{table}

% latex table generated in R 3.5.2 by xtable 1.8-4 package
% Tue Aug 13 13:49:18 2019
\begin{table}[!h]
\centering
\scalebox{1}{
\begin{tabular}{lllllllllllll}
  \hline
   m & \multicolumn{4}{c}{w = 0} & \multicolumn{4}{c}{w = 5} & \multicolumn{4}{c}{w = 10} \\ \cmidrule(lr){2-5}\cmidrule(lr){6-9}\cmidrule(lr){10-13}
  & MeC & MuC & MeU & MuU & MeC & MuC & MeU & MuU & MeC & MuC & MeU & MuU \\
 \hline
2 & 0.75 & 0.02 & 0.75 & 0.02 & 5.26 & 3.31 & 5.04 & 7.73 & 13.96 & 13.17 & 18.02 & 30.95 \\ 
  5 & 0.31 & 0.04 & 0.31 & 0.04 & 4.26 & 3.32 & 3.77 & 4.88 & 13.76 & 13.17 & 14.25 & 19.33 \\ 
  10 & 0.18 & 0.05 & 0.18 & 0.05 & 3.74 & 3.33 & 3.53 & 3.84 & 13.58 & 13.18 & 13.61 & 15.18 \\ 
  20 & 0.12 & 0.06 & 0.12 & 0.06 & 3.51 & 3.35 & 3.45 & 3.50 & 13.42 & 13.20 & 13.41 & 13.81 \\ 
   \hline
\end{tabular}
}
\caption{MISE as m increases, using true parameters, with J = 3.} 
\end{table}

% latex table generated in R 3.5.2 by xtable 1.8-4 package
% Tue Aug 13 13:49:18 2019
\begin{table}[!h]
\centering
\scalebox{1}{
\begin{tabular}{lllllllllllll}
  \hline
   N & \multicolumn{4}{c}{w = 0} & \multicolumn{4}{c}{w = 5} & \multicolumn{4}{c}{w = 10} \\ \cmidrule(lr){2-5}\cmidrule(lr){6-9}\cmidrule(lr){10-13}
  & MeC & MuC & MeU & MuU & MeC & MuC & MeU & MuU & MeC & MuC & MeU & MuU \\
 \hline
100 & 392.04 & 0.40 & 392.04 & 0.40 & 245.08 & 0.44 & 946.97 & 8.52 & 73.18 & 0.51 & 2492.00 & 33.28 \\ 
  200 & 177.30 & 0.19 & 177.30 & 0.19 & 198.40 & 0.21 & 431.76 & 8.07 & 59.15 & 0.34 & 1127.66 & 31.70 \\ 
  400 & 83.97 & 0.09 & 83.97 & 0.09 & 167.24 & 0.13 & 207.07 & 7.84 & 51.47 & 0.26 & 599.76 & 31.07 \\ 
  800 & 45.39 & 0.04 & 45.39 & 0.04 & 153.83 & 0.09 & 108.69 & 7.61 & 47.96 & 0.22 & 314.43 & 30.39 \\ 
   \hline
\end{tabular}
}
\caption{MISE as N increases, using true parameters, with J = 5.} 
\end{table}

% latex table generated in R 3.5.2 by xtable 1.8-4 package
% Tue Aug 13 13:49:18 2019
\begin{table}[!h]
\centering
\scalebox{1}{
\begin{tabular}{lllllllllllll}
  \hline
   m & \multicolumn{4}{c}{w = 0} & \multicolumn{4}{c}{w = 5} & \multicolumn{4}{c}{w = 10} \\ \cmidrule(lr){2-5}\cmidrule(lr){6-9}\cmidrule(lr){10-13}
  & MeC & MuC & MeU & MuU & MeC & MuC & MeU & MuU & MeC & MuC & MeU & MuU \\
 \hline
2 & 177.30 & 0.19 & 177.30 & 0.19 & 198.73 & 0.21 & 431.76 & 8.07 & 59.15 & 0.34 & 1127.66 & 31.70 \\ 
  5 & 54.93 & 0.24 & 54.93 & 0.24 & 96.32 & 0.27 & 100.12 & 4.60 & 43.51 & 0.37 & 264.40 & 17.75 \\ 
  10 & 27.38 & 0.32 & 27.38 & 0.32 & 47.51 & 0.32 & 32.93 & 3.03 & 31.71 & 0.42 & 62.47 & 11.08 \\ 
  20 & 11.37 & 0.44 & 11.37 & 0.44 & 20.66 & 0.43 & 13.52 & 2.34 & 19.97 & 0.50 & 21.54 & 7.65 \\ 
   \hline
\end{tabular}
}
\caption{MISE as m increases, using true parameters, with J = 5.} 
\end{table}

\end{document}
